# Supplementary material for: Recurrent Chunking Mechanisms for Long-Text Machine Reading Comprehension
Source: arXiv:2005.08056 source file (2020-05-19)
Supplement: Supplementary file 1 [file appendix.tex]

%\newpage
%\appendix
%\onecolumn
%\begin{center}
%	\Large Supplementary Material
%\end{center}

\section{Appendix}
%\subsection{Data Processing of CoQA and QuAC}
%We adopt data processing techniques \cite{bert2018} to deal with some questions whose answers do not exist in the document. We add a special token ``unknown'' to the end of each document. This token is the target answer span to unanswerable questions in both datasets. Since CoQA also contains questions with ``yes/no'' answers, we add a yes-no classifier to the answer extractor in the model, which predicts an answer to be ``yes'', ``no'' or a text span from a document. The classification loss is added to the answer loss $L_{\text{ans}}$ at the training stage.

\subsection{Analysis of different Stride Size in BERT-Large}
\label{stride_size_baseline}
We give the analysis on how the performance varied by choosing different stride sizes in BERT-Large model training and prediction, as in Table \ref{tab:stride_size_table}. An interesting observation is that smaller stride size in prediction doesn't always improve the performance, sometimes even hurts as shown in QuAC. It shows that BERT-Large performs badly on ensemble the answers from multiple chunks. Smaller stride size in model training also lead to the worse performance. A possible explanation is that smaller stride size would cause the significant distortion of training data distribution, the longer question-document pairs produces more training samples than short ones.

%\begin{figure*}[htbp!]
%\centering
%\includegraphics[width=0.95\textwidth]{chunk_example_jump.jpg}
%\caption{An example of the document segments generated by BERT-RCM.}
%\label{fig:chunk_example_jump}
%\vspace{-3mm}
%\end{figure*}

\begin{figure*}[htbp!]
\centering
\includegraphics[width=1.0\textwidth]{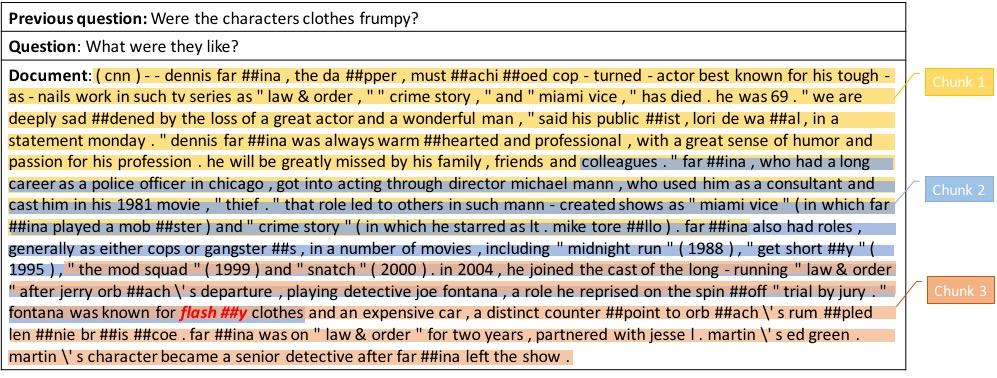}
\caption{Example 1 of generated document segments by BERT-RCM from a CoQA document.}
\label{fig:chunk_example_seq}
\end{figure*}

%\begin{figure*}[htbp!]
%\centering
%\includegraphics[width=1.0\textwidth]{chunk_example_jump.jpg}
%\caption{Example 2 of generated document segments by BERT-RCM from a CoQA document.}
%\label{fig:chunk_example_jump}
%\end{figure*}

\subsection{Case Studies}
\label{case_study}

We show an example of generated document segments by BERT-RCM from a CoQA document in the Figure \ref{fig:chunk_example_seq}. The ground truth answer ``flashy'' (tokenized as ``flash \#\#y'' by the BERT tokenizer) is colored in red. The document segments are generated by our chunking policy with LSTM recurrence. The model finds the first chunk irrelevant to the given question, and moves with the large stride size of $128$ tokens to the second chunk. The second chunk does not contain an answer, and the model again moves by $128$ tokens to the right. The answer is now captured by the third chunk, and with sufficient contexts around it. The chunking scorer predicts the three segments with $0.09$, $0.09$ and $0.91$  respectively, and the model extracts an answer span from the third doc-segment.
 
%We give the second example in Figure \ref{fig:chunk_example_jump}, where the model starts with the beginning of the document as the first segment, where the answer span is close to its right boundary. The model moves forwards $128$ tokens to include more right contexts and generates the second chunk. The stride size is a bit large since the answer is close to the left boundary of the second segment. The model then moves back to the left by $16$ tokens and obtains its third segment. The chunking scorer assigns the three segments with the scores $0.24$, $0.87$, and $0.90$, respectively. 

\begin{table*}[p]
\centering
%\resizebox{0.8\textwidth}{!}{
\begin{tabular}{l|cccc|cccc}
\toprule
Dataset & \multicolumn{4}{c|}{CoQA} & \multicolumn{4}{c}{QuAC} \\ 
\hline
BERT-Large ~\cite{bert2018} & \multicolumn{4}{c|}{Prediction Stride Size} & \multicolumn{4}{c}{Prediction Stride Size} \\ 
Training Stride Size  & 16 & 32 & 64 & 128 & 16  & 32 & 64 & 128 \\ 
\midrule
16 & 80.8 & 80.9 & 80.8 & 80.7 & 60.6 & 60.7 & 60.7 & 60.8 \\ 
\begin{tabular}[c]{@{}c@{}}  32\end{tabular} & 81.1 & 81.1 & 81.1 & 81.1 & 60.7 & 60.7 & 60.9 & 61.0 \\ 
\begin{tabular}[c]{@{}c@{}} 64\end{tabular} & \textbf {81.4} & \textbf{ 81.4} & \textbf{81.4} & 81.3 & 61.0 & 61.0 & \textbf{61.4} & \textbf{61.4} \\ 
\begin{tabular}[c]{@{}c@{}} 128\end{tabular} & 81.0 & 81.1 & 81.1 & 81.1 & 60.8 & 60.8 & 60.8 & 61.2 \\ 
\bottomrule
\end{tabular}%}
\caption{F1 score ($\%$) of BERT-Large with different training/prediction stride sizes on the CoQA and QuAC Datasets.}
\label{tab:stride_size_table}
\end{table*}
